# Supplementary material for: Strategic Arms with Side Communication Prevail Over Low-Regret MAB Algorithms
Source: arXiv:2408.17101 source file (2024-08-30)
Supplement: Supplementary file 1 [file 1_notation.tex]

\section{Notation}
Expectation $\lE$
